# Supplementary material for: Spline-based Reconstruction of Periodic Signals with Sparse Innovations
Source: arXiv:2111.14632 source file (2021-11-23)
Supplement: Supplementary file 2 [file DeclarationOfOriginalityZHAW.tex]

% Appendix: Declaration of Originality

\chapter{Declaration of Originality} % Main appendix title

\label{DeclarationOfOriginalityZHAW} % For referencing this appendix elsewhere, use \ref{AppendixA}

\includepdf[pages=-]{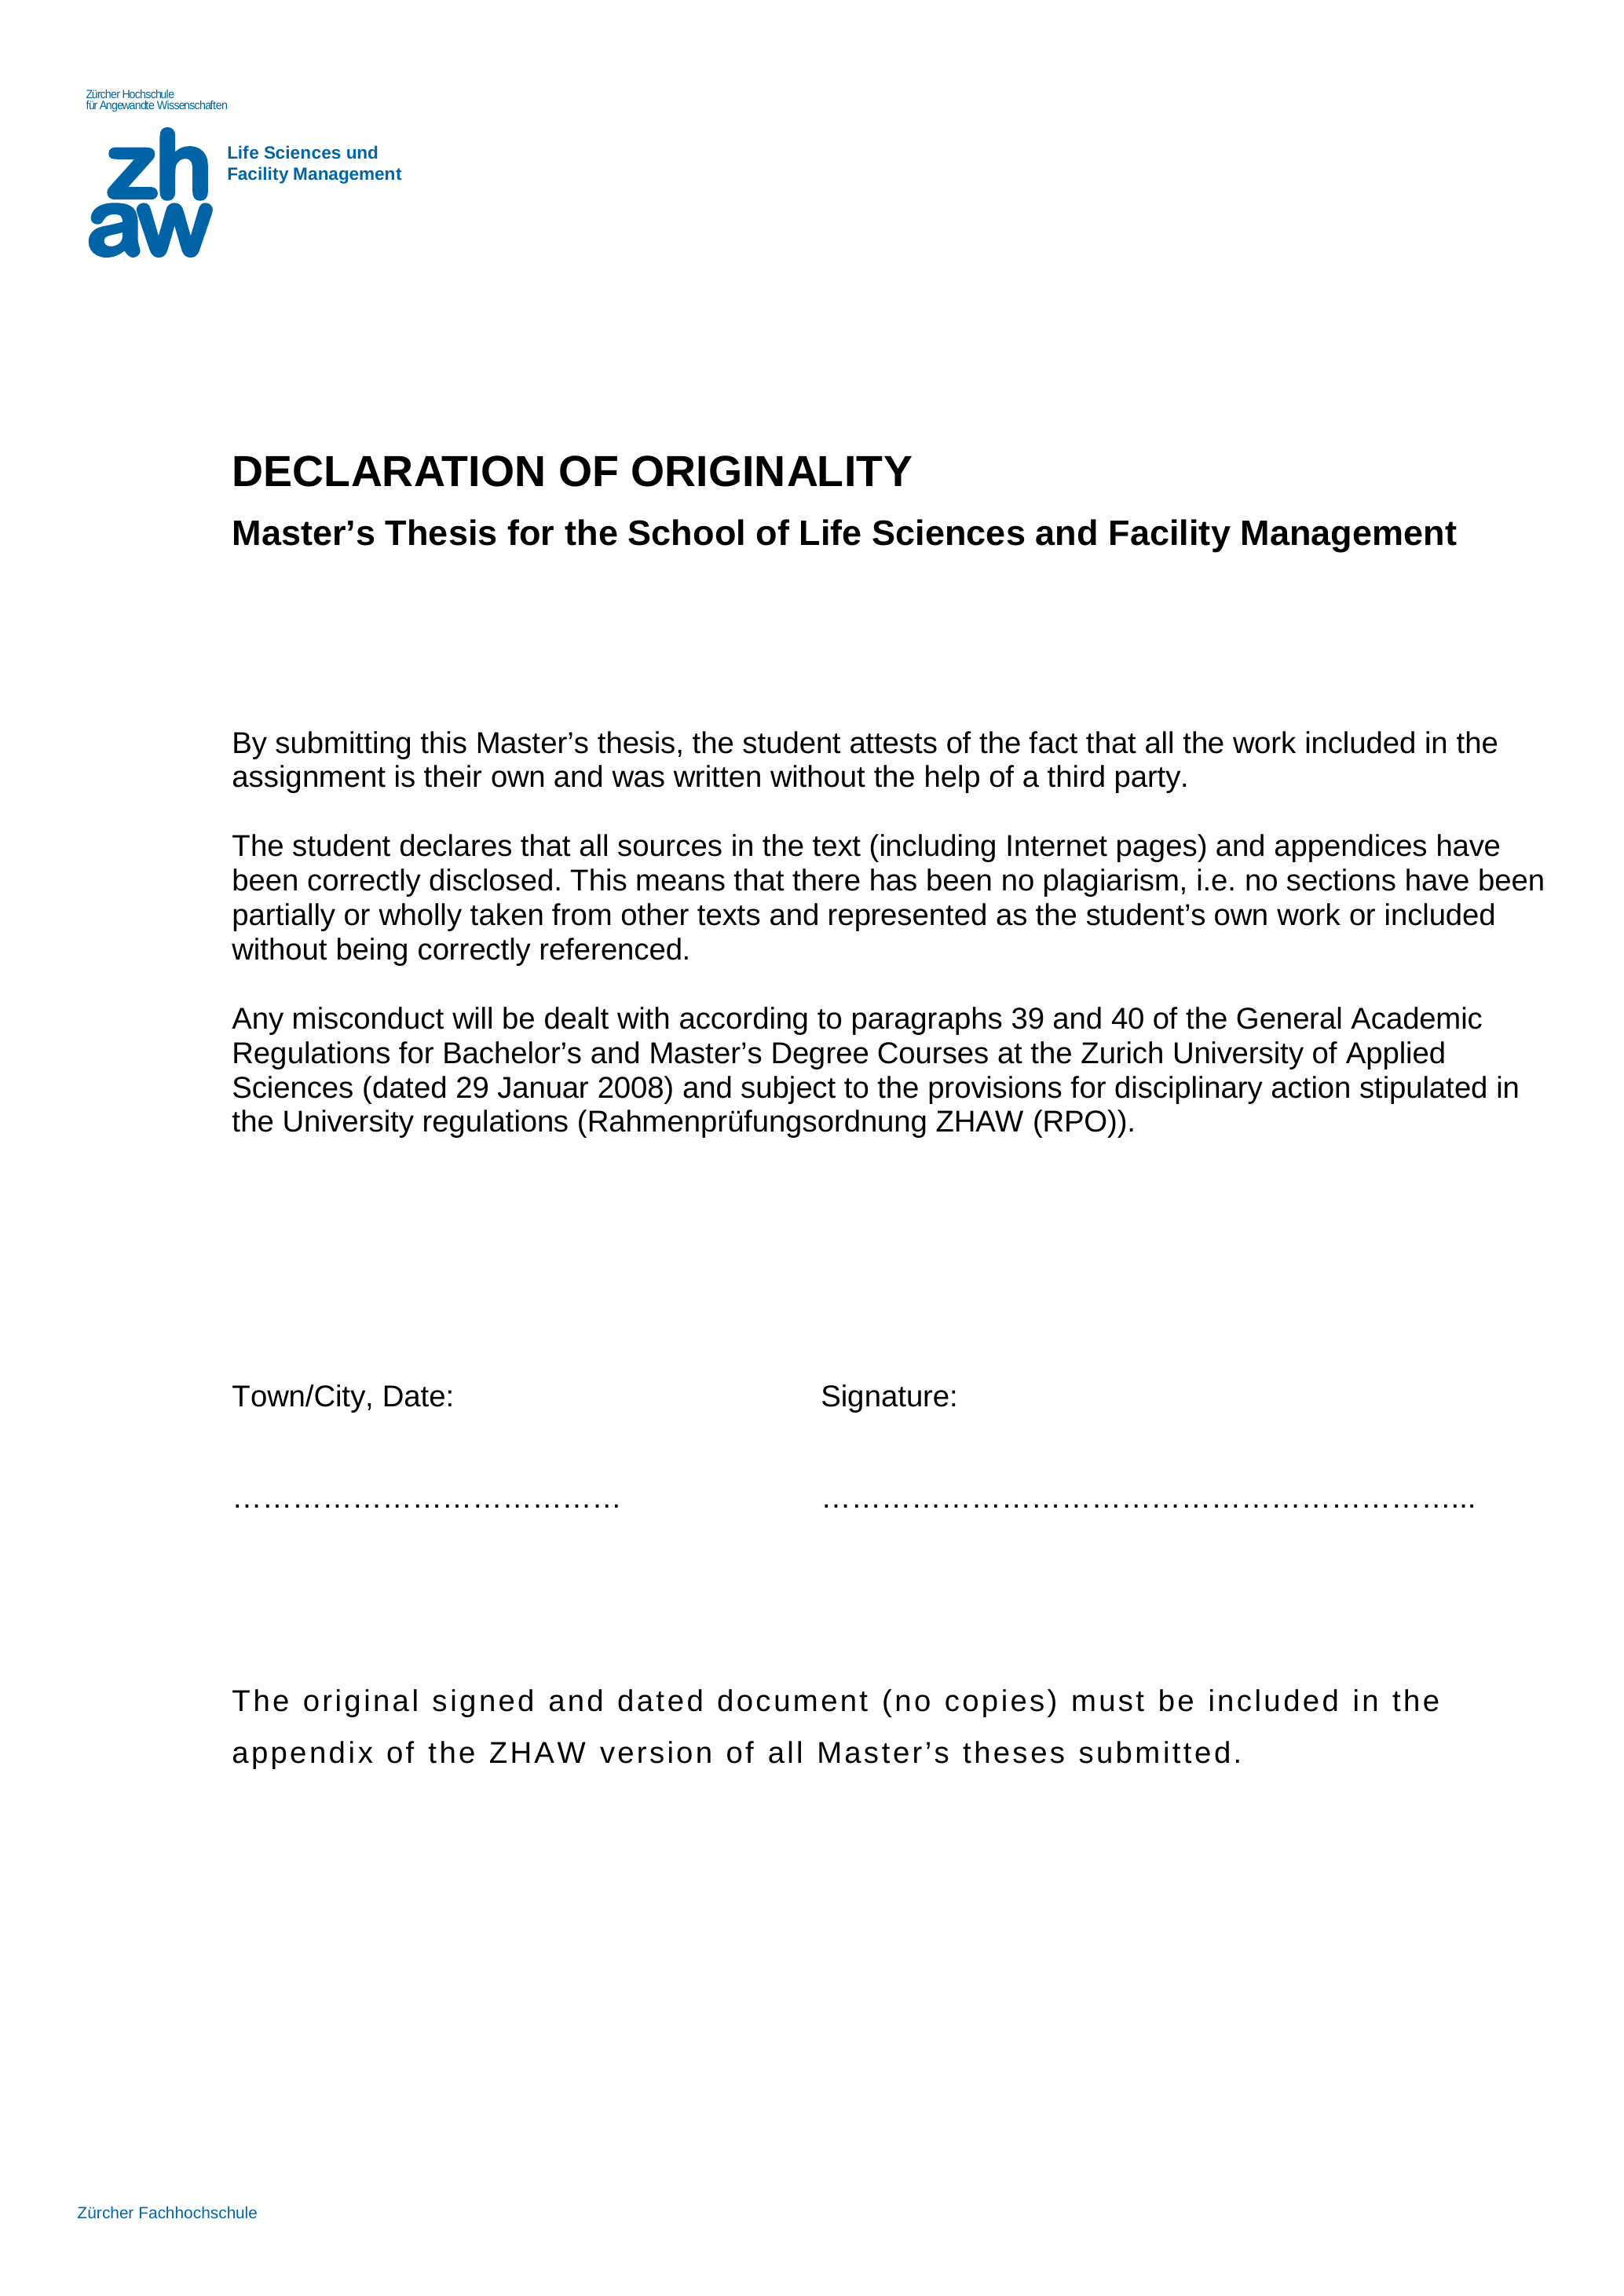}
