# Supplementary material for: Spline-based Reconstruction of Periodic Signals with Sparse Innovations
Source: arXiv:2111.14632 source file (2021-11-23)
Supplement: Supplementary file 3 [file AppendixTemplate.tex]

% Appendix Template

\chapter{Appendix Title Here} % Main appendix title

\label{ApendixX} % Change X to a consecutive letter; for referencing this appendix elsewhere, use \ref{AppendixX}

Write your Appendix content here.
